# Supplementary material for: Parallel Motif-Based Community Detection
Source: arXiv:2412.12382 source file (2024-12-16)
Supplement: Supplementary file 1 [file appendix.tex]

\section{More details on Related work }

Correlation clustering~\cite{bansal2004correlation} is a formulation of the graph clustering problem on signed graphs. Given a signed graph $G(V,E)$ and for each pair of nodes $(i,j)\in V$ two non-negative weights $w^+_{ij}$ and $w^-_{ij}$, the problem asks for a community assignment  that minimizes the total number of disagreements, i.e., 

\begin{equation}
    \label{eq:cc}
  \min_{c}  \sum_{i <j} w^-_{ij}\cdot \delta (c_u,c_v) +  w^+_{ij}\cdot (1-\delta (c_u,c_v)).
\end{equation}

\noindent In other words, a disagreement is a positive edge across two clusters or a negative edge within a cluster. While it is NP-hard to solve, there are constant approximations for the minimization version~\cite{bansal2004correlation,charikar2005clustering} and a polynomial time approximation scheme for the maximization version~\cite{bansal2004correlation} on complete graphs and $O(\log n)$-approximation on general graphs~\cite{demaine2006correlation} with possibly missing edges. 

Label propagation was adapted as a heuristic initially by~\cite{usha2007near}. The authors described a simple procedure where nodes adopt the most frequent community assignment among their neighbors until stable communities emerge. 
Soman and Narang~\cite{soman2011fast} speed up the method with multicore and GPU architecture, further improving the quality by introducing weights into the algorithm. 
Girvan-Newman algorithm~\cite{Girvan2002community} lies close to our framework. The algorithm computes the betweenness centrality of each edge and iteratively removes the edge with the highest centrality value. It takes the remaining connected components as output communities. It repeats the process until no edge is left and outputs a dendrogram of community structures. While performing well in finding communities on biological and social networks, this algorithm is limited to small-sized graphs only due to the complexity bottleneck from the betweenness centrality computation~\cite{abboud2014subcubic,williams2014faster}. 

\section{Figures and proofs for proposed method}

\subsection{Empirical observation}

\begin{figure*}[h]
	\centering
	\captionsetup[subfigure]{labelformat=empty}
	
	\begin{subfigure}[]{.15\linewidth}
		\centering
		\includegraphics[width=\linewidth]{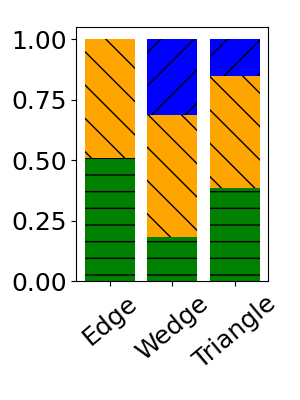}
		\caption{Gavin}
		\label{fig:m3-gavin}
	\end{subfigure} \hfill
	\begin{subfigure}[]{.15\linewidth}
		\centering
		\includegraphics[width=\linewidth]{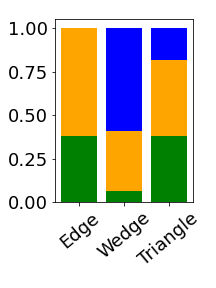}
		\caption{EXTE}
		\label{fig:m3-exte}
	\end{subfigure} \hfill
	\begin{subfigure}[]{.15\linewidth}
		\centering
		\includegraphics[width=\linewidth]{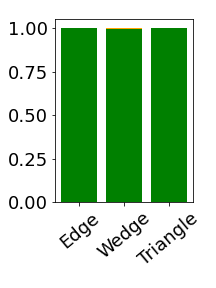}
		\caption{Amazon}
		\label{fig:m3-amazon}
	\end{subfigure} 
	\begin{subfigure}[]{.15\linewidth}
		\centering
		\includegraphics[width=\linewidth]{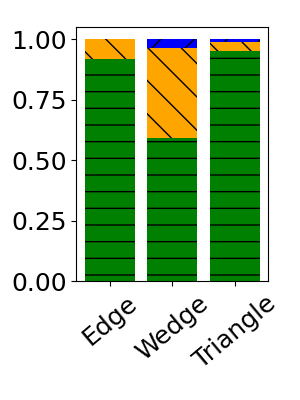}
		\caption{DBLP}
		\label{fig:m3-dblp}
	\end{subfigure} \hfill
	\begin{subfigure}[]{.15\linewidth}
		\centering
		\includegraphics[width=\linewidth]{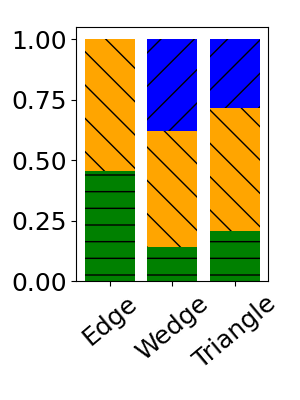}
		\caption{Youtube}
		\label{fig:m3-youtube}
	\end{subfigure} \hfill
	\begin{subfigure}[]{.15\linewidth}
		\centering
		\includegraphics[width=\linewidth]{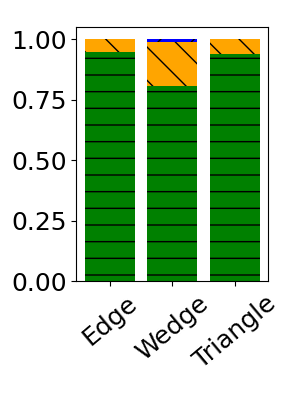}
		\caption{LiveJournal}
		\label{fig:m3-lj}
	\end{subfigure} 
	
	\begin{subfigure}[]{.2\linewidth}
		\centering
		\includegraphics[width=\linewidth]{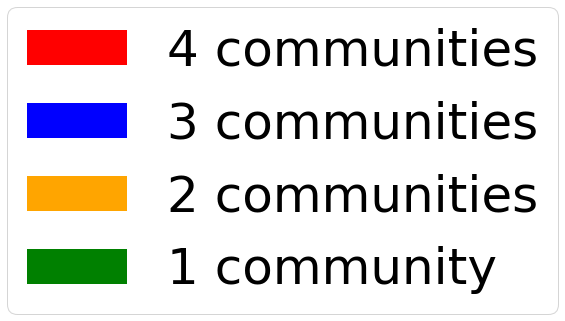}
		\caption{Legend}
		\label{fig:legend}
	\end{subfigure} \hfill
	\begin{subfigure}[]{.35\linewidth}
		\centering
		\includegraphics[width=\linewidth]{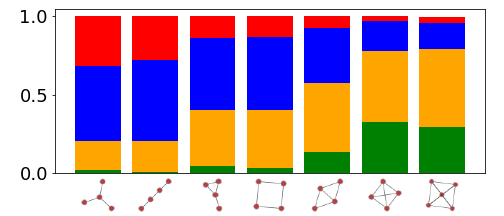}
		\caption{Gavin}
		\label{fig:m4-gavin}
	\end{subfigure} \hfill
	\begin{subfigure}[]{.35\linewidth}
		\centering
		\includegraphics[width=\linewidth]{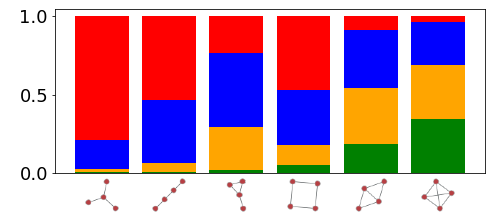}
		\caption{EXTE}
		\label{fig:m4-exte}
	\end{subfigure}
	\caption{\label{fig:motif_gt}Edges and motifs on groundtruth communities. In general, we see sparse motifs being cut more often by two or more communities.}
	
\end{figure*}

\subsection{Proof}
\label{appendix:proof}

\spara{\underline{ Proof of Theorem~\ref{thm:sbm}.} } Recall that   Tectonic removes  an edge $(u,v)$  if $\frac{t(u,v) }{d(u)+d(v)} < \delta $. Thus, we   define the tectonic score $Tec_{\delta}(u,v) = t(u,v) - \delta (d(u)+d(v))$. Table~\ref{tab:expected} provides a summary of the similarity score of each edge in expectation for the Tectonic and \TW scores, respectively, depending on the block participation of its endpoints $u,v$.  

\noindent {\it Tectonic:} Tectonic can recover the blocks in expectation if similarity scores of the edges across the two blocks and the edges within either block have no interleave, thus can be classified by some threshold. Assume there is such a threshold $\delta$ satisfies the condition.  This is equivalent to having $E[Tec_{\delta}(u,v)]>0$ for any $u,v\in B_i$, and $E[Tec_{\delta}(u,v)]<0$ for any $u\in B_1,v\in B_2$. Specifically, for any edge across two communities,

\begin{align*}
     E[Tec_{\delta}(u,v); u \in B_1, v \in B_2] &  = p_2q+2q^2-\delta(p_2+4q) <0  \rightarrow  \\ 
    \delta &> \frac{p_2q+2q^2}{p_2+4q} \overset{n \to \infty}{\longrightarrow} q
\end{align*}

\noindent For any edge induced by block $B_1$,

\begin{align*}
    E[Tec_{\delta}(u,v); u,v \in B_1] &  = 5q^2 -2\delta 3q
\end{align*}

\noindent By choosing $\delta>q$, 
\begin{align*}
    E[Tec_{\delta}(u,v); u,v \in B_1] & < -q^2<0
\end{align*}

\noindent Thus, the assumption is violated.

\underline{TW:} We will show that a range of thresholds exists to recover the communities in expectation. This is equivalent to having a positive gap in expectation between \TW of edges inside the block $B_1$ and across the two blocks. Specifically, the expected gap is $n(p_2-p_1) - 3n(p_1(q-p_1) + q(p_2-q))$. Given the assumption that $p_1=o(p_1)$, this gap value is dominated by $np_2$, making it positive. Therefore, TW can recover the communities in expectation.

 \begin{table}[]
    \centering
    \small
    \begin{tabular}{c|c|c|c|c|c}
         & \# triangles & \# wedges & $d_u+d_v$ & $\TW(u,v)$ & $Tec_{\delta}(u,v)$ \\ \hline
        \makecell{Inside\\ $B_1$} & $p_1^2+q^2$ & $2(p_1(1-p_1)+q(1-q))$ & $2(p_1+q) $ & \makecell{$3p_1^2-2p_1$\\ $+3q^2-2q$} & \makecell{$p_1^2+q^2$\\ $-2\delta (p_1+q)$} \\ \hline
        \makecell{Across\\ $B_1$, $B_2$} & $p_1q+p_2q$ & \makecell{$p_1(1-q)+p_2(1-q)+$ \\ $q(1-p_1)+q(1-p_2) $} & $p_1+p_2+2q$ & \makecell{$3p_1q+3p_2q$\\ $-p_1-p_2-2q$}  & \makecell{$p_1q +p_2q$\\ $-\delta (p_1+p_2+2q)$} \\
    \end{tabular}
    \caption{Expectation of various measures for each edge in an inhomogeneous SBM edge depending on the communities of its endpoints, normalized by $n$. We further assume $n-2 \approx n$ since we care about asymptotics. }
    \label{tab:expected}
\end{table}

\begin{proposition}\label{prop:equiv}
     Tectonic is an equivalent reparameterization of Jaccard edge similarity.
\end{proposition}

\begin{proof}
    For any threshold value $\delta$ for Jaccard edge similarity, an edge $(u,v)$ is removed if  the following holds: 
    \begin{align}
      \frac{t(u,v)}{\deg(u)+\deg(v)-t(u,v)}<\delta 
      \rightarrow (1+\delta)t(u,v)<\delta (\deg(u)+\deg(v))  \rightarrow \nonumber \\
        \frac{t(u,v)}{\deg(u)+\deg(v)}<\frac{\delta}{1+\delta} & \nonumber
    \end{align}

Observe that if we interpret $\delta$ as a probability, then the range of $\frac{\delta}{1 + \delta}$ is $[0,0.5]$. The equivalence is  immediately derived from the bijectiveness of the function $f(\delta)=\frac{\delta}{1+\delta}$ in the interval $\delta \in [0,1]$. {\bf QED}

\end{proof}

\subsection{Visualization}\label{appendix:visual}

We show in Figure~\ref{fig:add_syncomp_visual} that both $K_3$ and spectral clustering are not able to recover the communities in SBM. Louvain, while lacking theoretical guarantee, almost fully recovers the blocks.

\begin{figure}
    \centering
    \begin{subfigure}[]{0.25\linewidth}
        \centering
        \includegraphics[width=\linewidth]{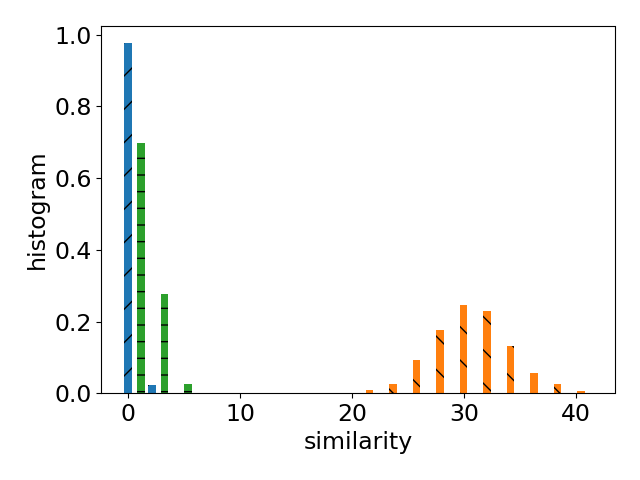}
        \caption{$K_3$}
    \end{subfigure} \hfill
    \begin{subfigure}[]{0.25\linewidth}
        \centering
        \includegraphics[width=\linewidth]{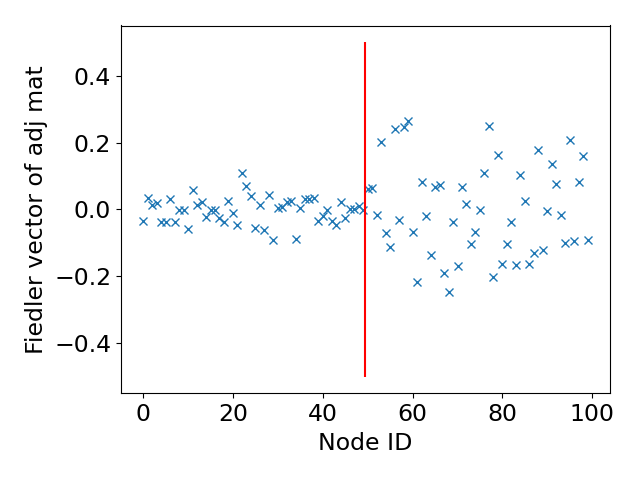}
        \caption{Spectral clustering}
    \end{subfigure} \hfill
    \begin{subfigure}[]{0.25\linewidth}
        \centering
        \includegraphics[width=\linewidth]{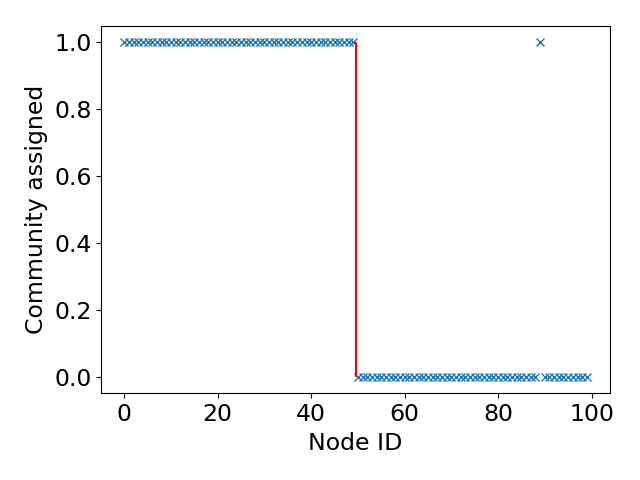}
        \caption{Louvain}
    \end{subfigure}
    \caption{Comparison of community detection methods in terms of output quality on an imbalanced SBM.}
    \label{fig:add_syncomp_visual}
\end{figure}

\section{Experiments}
\label{appendix:exp}

\subsection{Evaluation framework}\label{appendix:eval}

\textit{Remark:} Unlike the one proposed in \cite{Tsourakakis2017scalable}, the evaluation framework we use does not guarantee the monotonicities of precision and recall w.r.t. the resolution. In fact, we show in Figure~\ref{fig:eval_motivate} that such monotonicities should not exist when evaluating graph partitions with overlapping groundtruth communities. Given the four groundtruth communities, there are two perfect ways to partition the graph, i.e., partition them into three squares to match with $\{C_1,C_2,c_3\}$ or return the whole graph to match with $\{C_4\}$. In the example, these two perfect structures are output by an algorithm with high and low resolutions, and both should receive full precision and recall. On the other hand, the defective output with the mid-resolution deserves a lower evaluation score. Our designed evaluation framework is able to measure the performance accurately in these cases.

\begin{figure}
    \centering
    \input{figs/ticks/eval_motivation}
    \caption{Left: A toy graph with four overlapping groundtruth communities. Right: Brown circles are the community structures detected with resolutions set to be high, mid, and low. }
    \label{fig:eval_motivate}
\end{figure}

\textbf{Groundtruth communities for SNAP datasets.} For each SNAP dataset, we evaluate any result based on the whole set of groundtruth communities, except the ones with a size of less than 3. Note this is different from the previous studies that usually take the top 5000 communities as the ground truth. This is because the metrics used in~\cite{yang2012define} to find top communities are separability, density, cohesiveness, and clustering coefficient. Such measurements naturally constrain the community structures to follow their hypothesis and lose the value of using ground truth data. For example, Figure~\ref{fig:dblp_com_density_compare} shows more than one-third of the top 5000 communities selected in the three datasets are cliques or near-cliques, i.e., subgraphs with edge densities close to 1. In contrast, the real ground truth communities have edge densities ranging more widely. Therefore, the downstream evaluations favor methods that generate clique-like community structures. 

\begin{figure}
    \centering
    \begin{subfigure}[]{0.3\linewidth}
        \centering
        \includegraphics[width=\linewidth]{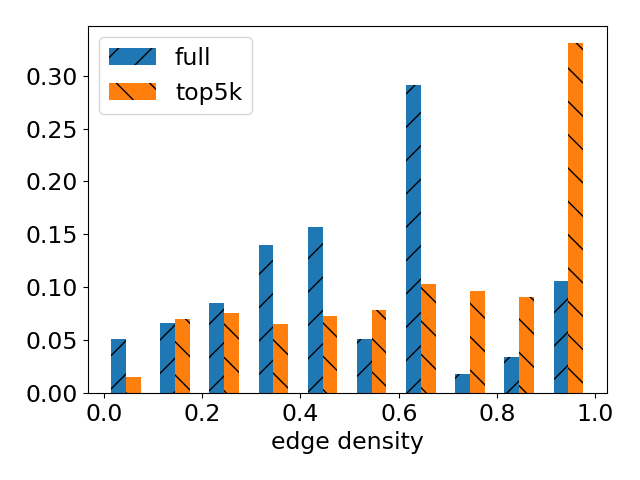}
        \caption{}
    \end{subfigure} \hfill
    \begin{subfigure}[]{0.3\linewidth}
        \centering
        \includegraphics[width=\linewidth]{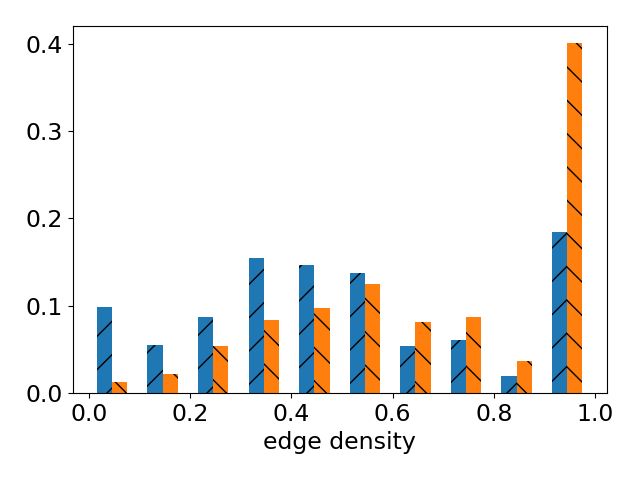}
        \caption{}
    \end{subfigure} \hfill
    \begin{subfigure}[]{0.3\linewidth}
        \centering
        \includegraphics[width=\linewidth]{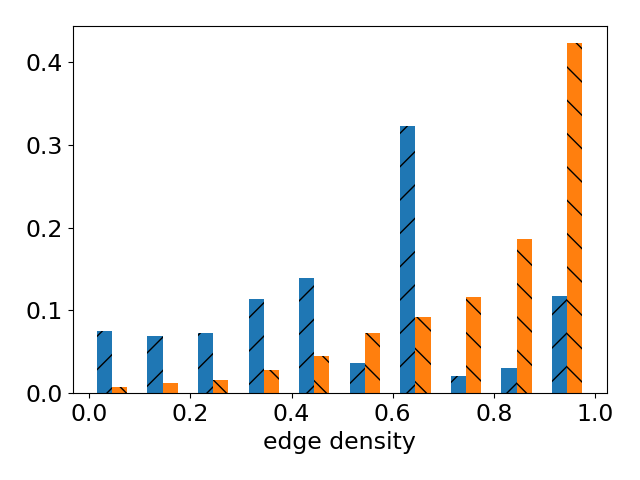}
        \caption{}
    \end{subfigure}
    \caption{Histograms of community densities of (a) Amazon, (b) DBLP, (c) LiveJournal.}
    \label{fig:dblp_com_density_compare}
\end{figure}

\subsection{Details of baselines and parameter settings}

We apply the following methods as baselines in the experiments. Resolutions are tuned by parameters listed in Table~\ref{tab:params}. 

\begin{itemize}
    \item {\it Parallel correlation clustering (PCC)}~\cite{shi2021scalable} . This method greedily optimizes the LambdaCC objective proposed by Veldt et al.~\cite{veldt2018correlation}. Authors optimize their parallel framework with various options, e.g., asynchronous setting, multi-level refinement, etc. 
    \item {\it Parallel modularity optimization (PMod)}~\cite{shi2021scalable}. The framework of Shi et al.~\cite{shi2021scalable} also supports optimizing in parallel a modularity objective proposed by Reichardt and Bornholdt~\cite{reichardt2006Statistical}, which is a generalization of the standard modularity metric used by Louvain~\cite{Girvan2002community}. 
    \item {\it Label propagation communities (LPC)}. We use the implementation provided by Networkx, which is a semi-synchronous label propagation method~\cite{cordasco2010community}.
    \item {\it Infomap}. The package provided by~\cite{mapequation2023software} is written in C++ and wrapped with Python APIs.
    \item {\it Spectral clustering\footnote{\url{https://scikit-learn.org}.} (Spec)}~\cite{ng2001spectral}, and higher-order spectral clustering using triangles (H-Spec)~\cite{benson2016higher}.
\end{itemize}

\begin{table}[th]
    \centering
        \caption{  \label{tab:params}Parameters and their respective ranges explored for each method to control resolution when evaluating the precision-recall tradeoff.}
    \begin{tabular}{c|c|c} 
      Method   &  Parameter & Range (start, end, step size) \\ \midrule
       TW  & $\delta$ & (-30,0,2) \\ 
       Tectonic  & $\delta$ & (0,0.3,0.02) \\ 
       $K_3$  & $\delta$ & (0,15,1) \\ 
       PCC  & $\lambda$ & (0.01,0.96,0.05) \\ 
       PMod  & $\gamma$ & $2m\times (0.1,1,0.05)$ \\ 
       Spectral clustering & \# of clusters & (100,1300,300)
    \end{tabular}

\end{table} 

\subsection{Additional results}

\begin{figure}
    \centering
    \begin{subfigure}[]{0.25\linewidth}
        \centering
        \includegraphics[width=\linewidth]{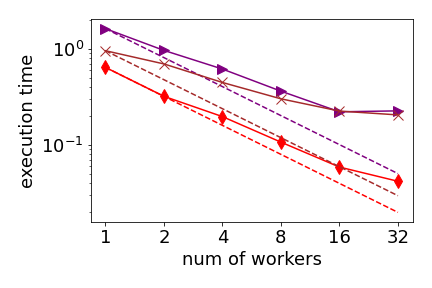}
        \caption{DBLP}
    \end{subfigure}  \hfill
    \begin{subfigure}[]{0.25\linewidth}
        \centering
        \includegraphics[width=\linewidth]{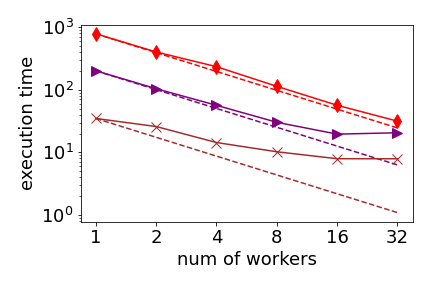}
        \caption{Orkut}
    \end{subfigure} 
    \caption{Execution time of \TW and two parallel baselines.}
    \label{fig:add_scale_real}
\end{figure}

\begin{figure}
    \centering
    \begin{subfigure}[]{0.3\linewidth}
        \centering
        \includegraphics[width=\linewidth]{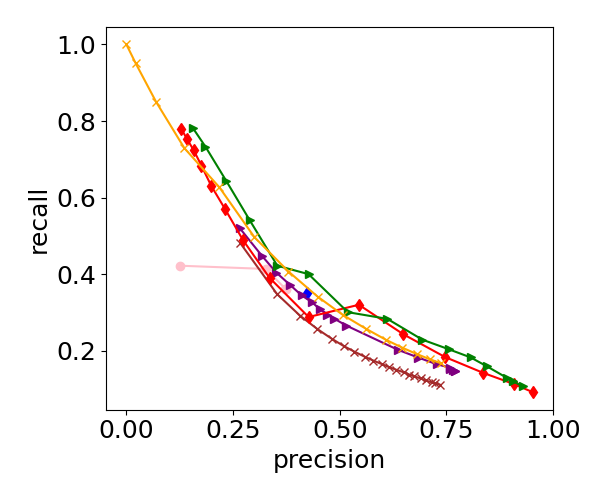}
        \caption{DBLP}
    \end{subfigure}  
    \begin{subfigure}[]{0.3\linewidth}
        \centering
        \includegraphics[width=\linewidth]{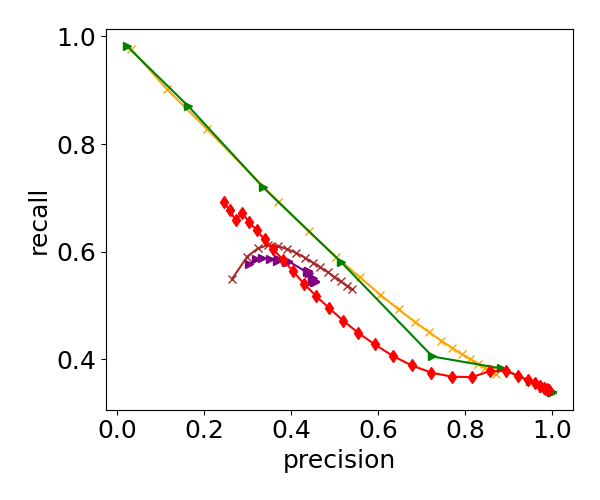}
        \caption{Orkut}
    \end{subfigure}  \hfill
    \caption{Precision recall tradeoff on SNAP datasets.}
    \label{fig:add_pre_recall}
\end{figure}
